# Supplementary material for: Abnormal $phase$ flip in coherent phonon oscillations of Ca$_2$RuO$_4$
Source: arXiv:1808.06026 source file (2018-08-18)
Supplement: Supplementary file 1 [file supplemental_materials.pdf]

*Supplemental material* for

# Abnormal *phase*-flip in coherent phonon oscillations of $Ca_2RuO_4$

Min-Cheol Lee[1, 2], Choong H. Kim[1, 2], Inho Kwak[1, 2], J. Kim[3], S. Yoon[3], Byung Cheol Park[1, 2], Bumjoo Lee[1, 2], F. Nakamura[4], C. Sow[5], Y. Maeno[5], T. W. Noh[1, 2*] & K. W. Kim[6†]

[1]*Center for Correlated Electron Systems, Institute for Basic Science (IBS), Seoul 08826, Republic of Korea*

[2]*Department of Physics and Astronomy, Seoul National University, Seoul 08826, Republic of Korea*

[3]*Department of Physics and New Renewable Energy Research Center (NREC), Ewah Womans University, Seoul 03760, Republic of Korea*

[4]*Department of Education and Creation Engineering, Kurume Institute of Technology, Fukuoka 830-0052, Japan*

[5]*Department of Physics, Graduate School of Science, Kyoto University, Kyoto 606-8502, Japan*

[6]*Department of Physics, Chungbuk National University, Cheongju, Chungbuk 28644, Republic of Korea*

Corresponding authors:

[*]twnoh@snu.ac.kr, [†]kyungwan.kim@gmail.com

## 1. Fluence dependence of the coherent phonon oscillations

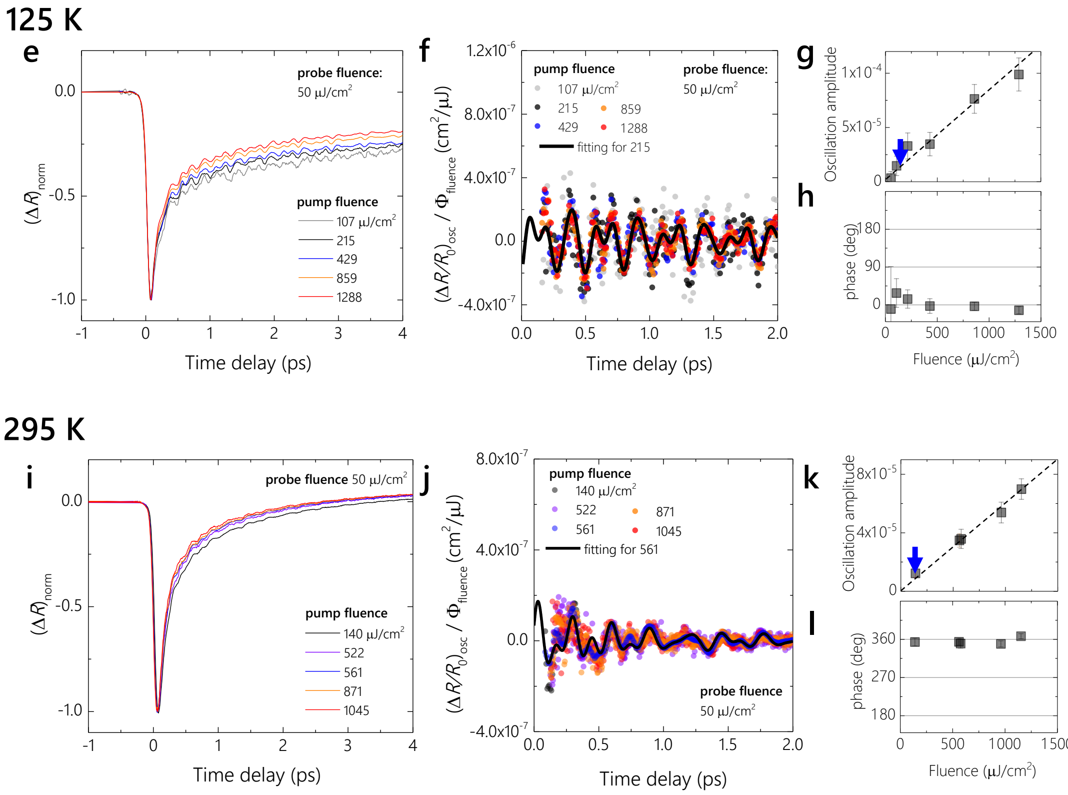


**Figure S1**. Fluence dependent reflectivity changes and coherent oscillations at 125 K (< $T_{OO}$ = 260 K) and 295 K (> $T_{OO}$). **(a), (e)** Photo-reflectivity normalized by the maximum value under a pump fluence of up to ~ 1 mJ/cm$^2$. **(b), (f)** Extracted oscillation components and a fitting curve composed of four $A_g$ modes. **(c), (g)** Amplitude and **(d), (h)** *phase* values of the lowest $A_g$ phonon oscillations under various pump fluences. There is a clear linear response up to ~ 1 mJ/cm$^2$. The blue arrow in (c) indicates the pump fluence used for the measurements in the manuscript.

The oscillation-*phase* of the lowest $A_g$ phonon mode does not depend on the light fluence. Figure S1 shows the fluence dependent data of the coherent phonon oscillations at different temperatures, i.e., 125 K (< $T_{OO}$) and 295 K (> $T_{OO}$), with various pumping fluences. In particular, the oscillation-*amplitude* of the lowest $A_g$ mode clearly shows a linear response, and the oscillation-*phase* remains the same even at a pumping fluence of up to ~ 1 mJ/cm$^2$. Despite the linear response of the coherent phonon oscillations, we present data measured at pump and probe fluences of 140 and 80 μJ/cm$^2$, respectively, to minimize heating effects and remain close to a linear response region of the electronic response.

## 2. Fits to relaxation dynamics

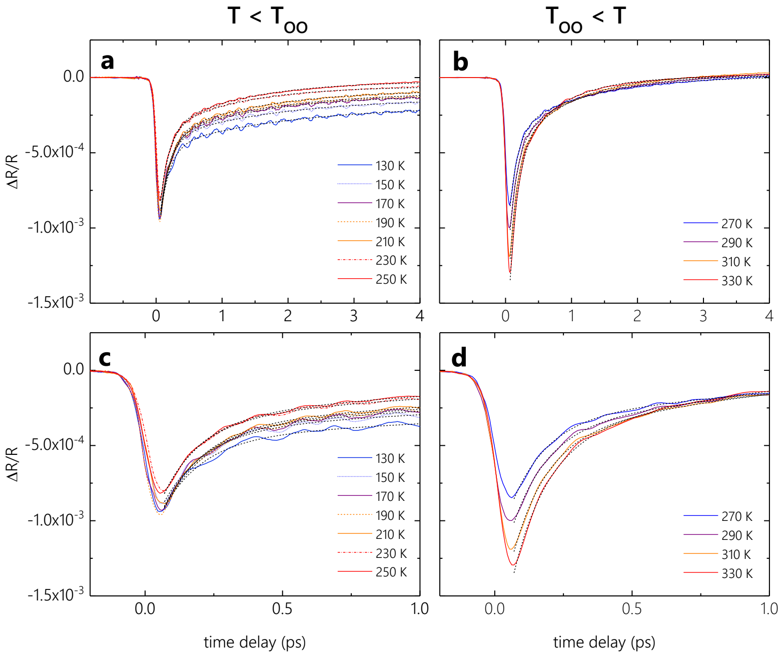


**Figure S2**. Relaxation fits (black dotted lines) of two-exponential decay model for temperature dependent reflectivity changes (colored lines).

We analyze the oscillatory components due to coherent phonons after subtracting double exponential decay function fits to the electronic response. Figure S2 shows the reflectivity change within a few picoseconds and relaxation fits at various temperatures. The overall electronic response does not show an abrupt change across $T_{OO}$, where such a change could influence the coherent oscillations under discussion.

## 3. Raman spectra

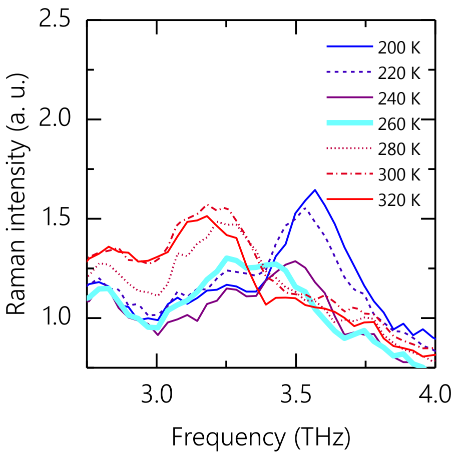


**Figure S3**. (c) Raman spectra of the lowest $A_g$ phonon mode that also shows a suppression in amplitude at 260 K.

We perform Raman scattering measurements to reveal the temperature dependent anomaly across 260 K in equilibrium state. Although there is little discrepancy in peak frequencies obtained from the Raman data and the coherent phonon oscillations which might be due to experimental errors, the Raman intensity of the lowest $A_g$ phonon also shows the suppression at 260 K as shown in Fig. S3.

## 4. Temperature dependence of absorption

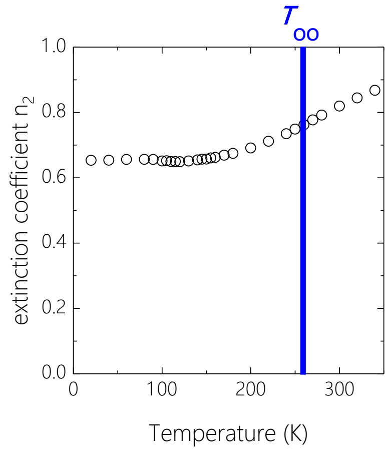


**Figure S4**. Temperature dependence of the extinction coefficient at 1.55 eV in $Ca_2RuO_4$

The absorption at 1.55 eV does not show a temperature dependent anomaly across $T_N$ = 260 K, as shown in Fig. S4. We measured the *ab*-plane reflectivity spectra from 20 K to 340 K over a photon energy region between 0.7 and 5 eV using spectroscopic ellipsometry. Although there is a gradual change in the absorption above $T \sim 200$ K, absorption of the pump photon energy remains strong across $T_{OO}$.

## 5. A possible generation mechanism of the lowest $A_g$ phonon in $Ca_2RuO_4$

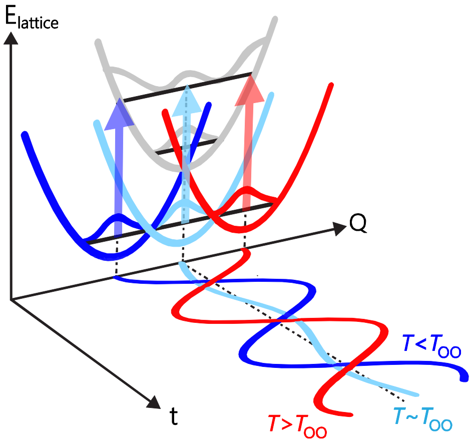


**Figure S5**. (color online) Schematic diagram of a possible generation mechanism of the lowest $A_g$ phonon oscillation in $Ca_2RuO_4$. Depending on the lattice structures at various temperatures, the oscillation-*phase* could change even with flipping across $T_{OO}$. Arrows indicate the optical transition resulting from 1.55 eV pumping. Vibrational functions of $n = 0$ and $n = 1$ modes are also displayed in each lattice potential.

We schematically describe one of the possible ways to induce the phase-flip across $T_{OO}$ as shown in Fig. S4. As discussed in the main text, a *phase*-flip can be obtained by a sign change in $(\partial R/\partial Q)$ or $\delta Q$ because $\Delta R_{CP} = (\partial R/\partial Q)\delta Q$ [3,4]. In $Ca_2RuO_4$, if the equilibrium lattice coordinate $Q_0$ shifts depending on temperature, the flip of the reflectivity modulations may occur because $\delta Q = Q_0^{ex} - Q_0$ gradually changes its sign across $T_{OO}$, as shown in Fig. S5. On the other hand, the *phase*-flip also could occur when $(\partial R/\partial Q)$ changes the sign while the sign of $\delta Q$ is invariant.

## 6. Determination of time zero delay

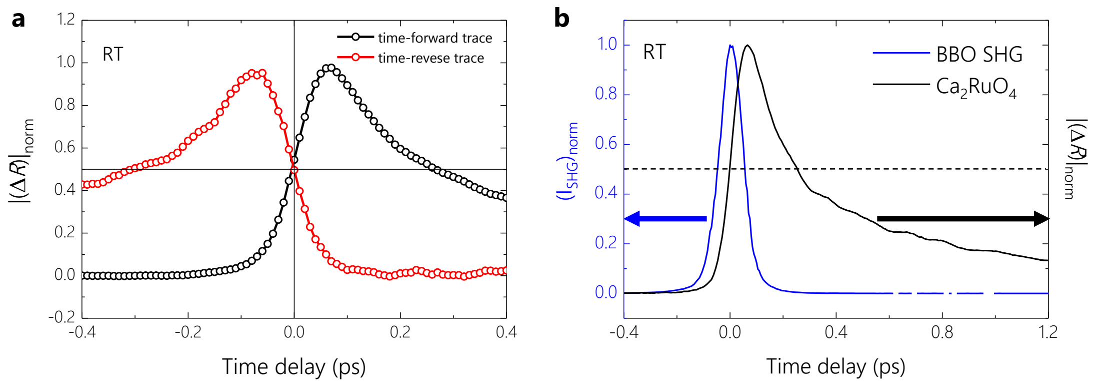


**Fig. S5**. (a) Pump-probe data of $Ca_2RuO_4$ obtained by optical chopping of the pump beam (black) and probe beam (red). (b) Second harmonic signal generated by pump and probe pulses from a beta barium borate (BBO) (blue) crystal and the photo-reflectivity change of $Ca_2RuO_4$ (black). We measure all data at room temperature, and display here with the absolute values normalized by the maximum change for easy comparison.

Precise determination of time zero, i.e. the zero reference for time delay measurements, is necessary to analyze the oscillation-*phase*. We determine the time zero from (a) forward and backward traces of the pump–probe signal, and (b) the cross correlation of pump and probe pulses as shown in Fig. S5. In the former case, we chop the pump beam in the forward trace (black curve), and the probe beam in the backward trace (red curve) [3]. The latter case is obtained by the second-harmonic signals of the pump and probe pulses. Please note that although the time widths of both the pump and probe pulses measured by a commercial autocorrelator (model: PulseScout; Newport Corporation) are 30 fs, the width of the cross correlation signal is larger because we have used a thick (0.5 mm) beta barium borate (BBO) crystal for second-harmonic generation (SHG) measurements. The time error due to the specification of the delay stage is about 3 fs considering reproducibility of within 0.5 μm (model: M-IMS600LM; Newport Corporation). In practice, the maximum onset time variation of the repeated measurements over 10 times is 10 fs, and this corresponds to a 15° error in the oscillation-*phase* values.

## 7. Fits to coherent phonon oscillations

We fit the $A_g$ coherent phonon oscillations using a damped harmonic oscillating model:

$$R_{CP}(t) = -\Sigma_i A_i \cos(2\pi f_i + \phi_i) \exp(-t/\tau_i),$$

where $A_i$, $f_i$, $\phi_i$, and $\tau_i$ are the amplitude, frequency, initial *phase*, and damping time of the $A_g$ symmetric modes, respectively. We mainly consider four oscillators corresponding to the equilibrium $A_g$ Raman modes [1,2]. Fourier transform spectra in Fig. 2(b) barely reveal the two $A_g$ modes around 5.8~6 THz; however, DFT calculations that these two modes are distinct but with similar resonant energy. Therefore, we consider four modes including both modes around 6 THz in our model. The anomalies in *phase* and amplitude are first obtained by fitting all parameters of the four modes. Figure S6(a) and (b) show the fitting results. The oscillatory components of the 3.8-THz mode in Fig. S6(a) are obtained by subtracting the fitting functions of other three modes from the raw data. Figure S7 shows the oscillation-*phases* of all four modes in the case of fitting without fixed *phase*s for all $A_g$ modes. We find that not only the lowest frequency mode, but also other modes show small variation. However, the fitting error bars are very large for the parameters of the other higher-frequency modes (please note that the error bars here do not include the measurement errors). We also notice that the oscillation amplitudes of other modes are relatively small and their temperature dependences are not systematic; therefore, care should be taken when interpreting the outcome. Based on these results, one may suspect that such non-systematic fitting parameters could produce a systematic artifact in the other fitting parameter, that is, in the oscillation-*phase* of the 3.8 THz mode.

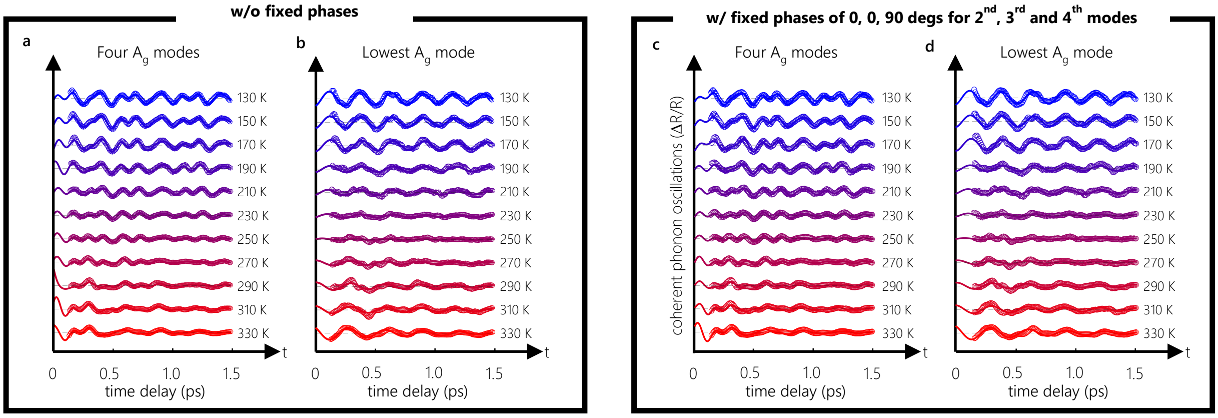


**Figure S6**. Fits for the lowest and higher frequency $A_g$ coherent phonon modes (a, b) without and (c, d) with fixation of the oscillation-*phase*s of higher frequency modes. (a) and (c) show all oscillating components, and (b) and (d) show the lowest frequency component and fit functions after subtracting the fit functions of the other higher modes.

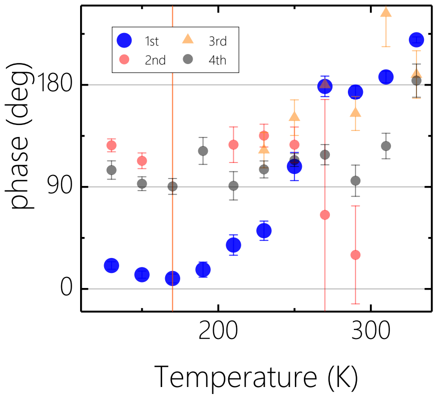


**Figure S7.** Oscillation-*phases* from the fits to the oscillatory signal.

Because the oscillation-*phase* is usually considered to be a robust quantity of either 0 or 90°, depending on the generation mechanism, we repeat the fitting with all of the oscillation-*phases* being fixed except the 3.8-THz mode. We try oscillation-*phases* of (0, 0, 0) degrees, (90, 90, 90) degrees, and (0, 0, 90) degrees for 5.8-, 6.2-, 7.5-THz modes. Among them, we find that the condition of (0, 0, 90) degrees for (5.8, 6.2, 7.5) THz modes gives the best fitting quality; the results are shown in Fig. S6(c), (d). We find that the overall fitting qualities, with or without fixing of oscillation-*phases*, are comparable.

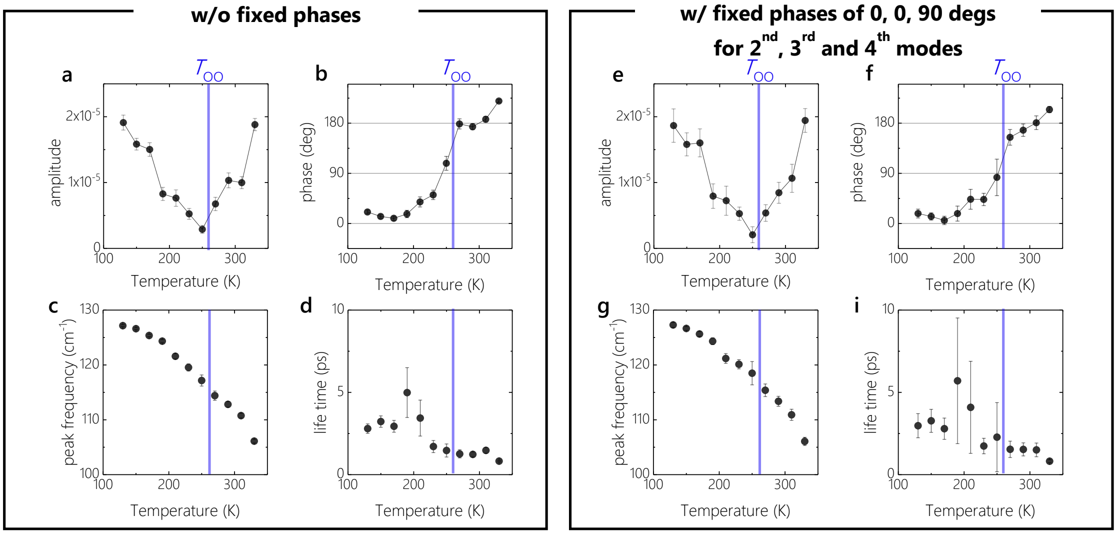


**Figure S8**. Fitting parameters of amplitude, *phase*, peak frequency and lifetime of the lowest frequency $A_g$ mode extracted by the damped harmonic oscillator models (a–d) without and (e–h) with fixing of the oscillation-*phases* of higher frequency modes. It is clear that the *phase* values of the other modes do not influence the temperature dependent anomalies of the 3.8-THz $A_g$ mode.

Figure S8 shows the detailed parameters of the 3.8 THz mode for the two fitting results. It becomes clear that the anomalies in the 3.8 THz phonon modes do not depend on the fitting parameters of the other modes. Because it does not make sense to allow the *phases* of all modes to change randomly, we use this fitting result with fixing of the oscillation-*phases* of other modes for further discussions in the manuscript.

## Reference


[1] H. Rho, S. L. Cooper, S. Nakatsuji, H. Fukazawa, and Y. Maeno, Phys. Rev. B **71**, 245121 (2005).

[2] S.-M. Souliou, J. Chaloupka, G. Khaliullin, G. Ryu, A. Jain, B. J. Kim, M. Le Tacon, and B. Keimer, Phys. Rev. Lett. **119**, 067201 (2017).

[3] H. J. Zeiger, J. Vidal, T. K. Cheng, E. P. Ippen, G. Dresselhaus, and M. S. Dresselhaus, Phys. Rev. B **45**, 768 (1992).

[4] T. Stevens, J. Kuhl, and R. Merlin, Phys. Rev. B **65**, 144304 (2002).
